# Supplementary material for: Multifunctional Composites for Elastic and Electromagnetic Wave Propagation
Source: arXiv:1908.06662 ancillary file (2020-05-12)
Supplement: Supplementary file 1 [file SupplementaryInformation.pdf]

# Supplementary Information: Multifunctional Composites for Elastic and Electromagnetic Wave Propagation

Jaeuk Kim[1] and Salvatore Torquato[1,2,3,4,*]
1. Department of Physics, Princeton University, Princeton, New Jersey 08544, USA
2. Department of Chemistry, Princeton University, Princeton, New Jersey 08544, USA
3. Princeton Institute for the Science and Technology of Materials, Princeton University, Princeton, New Jersey 08544, USA
4. Program in Applied and Computational Mathematics, Princeton University, Princeton, New Jersey 08544, USA
* torquato@princeton.edu; http://chemlabs.princeton.edu

## I. SPECTRAL DENSITY

We explain the definition of the spectral density $\tilde{\chi}_{_V}(\boldsymbol{Q})$ and how to measure it experimentally. Then we discuss how to numerically compute $\tilde{\chi}_{_V}(\boldsymbol{Q})$ of a dispersion consisting of hard (nonoverlapping) spheres. For a two-phase heterogeneous system in $d$-dimensional Euclidean space $\mathbb{R}^d$, the autocovariance function is defined as

$$\chi_{_V}(\boldsymbol{r}) \equiv S_2^{(i)}(\boldsymbol{r}) - {\phi_i}^2, \tag{S1}$$

where $S_2^{(i)}(\boldsymbol{r})$ and $\phi_i$ are the two-point correlation function and the volume fraction of phase $i$, respectively. The autocovariance function $\chi_{_V}(\boldsymbol{r})$ is identical for each phase and converges to zero as $|\boldsymbol{r}|$ increases when the system does not have long-range order [1]. The spectral density $\tilde{\chi}_{_V}(\boldsymbol{Q})$ is the Fourier transform of $\chi_{_V}(\boldsymbol{r})$ at a wavevector $\boldsymbol{Q}$ and is a nonnegative real-valued function of $\boldsymbol{Q}$. Since $\chi_{_V}(\boldsymbol{r})$ is dimensionless, the spectral density has a dimension of an inverse of volume. In scattering experiments, the spectral density $\tilde{\chi}_{_V}(\boldsymbol{Q})$ can be directly obtained from the scattering intensity [2] when $\boldsymbol{Q}$ is the scattering momentum transfer, i.e., $\boldsymbol{Q} = \boldsymbol{k}_{\text{scat}} - \boldsymbol{k}_{\text{inc}}$, where $\boldsymbol{k}_{\text{scat}}$ and $\boldsymbol{k}_{\text{inc}}$ are the wavevectors of scattered and incident waves, respectively.

Now we consider a dispersion in a periodic fundamental cell $\mathcal{F}$ in $d$-dimensional Euclidean space $\mathbb{R}^d$ that contains $N$ nonoverlapping spheres of radii $a_1,\cdots,a_N$ and positions $\boldsymbol{r}_1,\cdots,\boldsymbol{r}_N$. Then, the spectral density can be directly computed from the following formula [1]:

$$\tilde{\chi}_{_V}(\boldsymbol{Q}) = \frac{1}{V_{\mathcal{F}}}\left|\sum_{j=1}^{N} \tilde{m}(|\boldsymbol{Q}|;a_j)\, e^{-i\boldsymbol{Q}\cdot\boldsymbol{r}_j}\right|^2, \tag{S2}$$

where $V_{\mathcal{F}}$ is the volume of this fundamental cell, $\tilde{m}(Q;a) \equiv (2\pi a/Q)^{d/2}\, J_{d/2}(Qa)$, and $J_\nu(x)$ is the Bessel function of order $\nu$. Here, a wavevector $\boldsymbol{Q}$ corresponds to the reciprocal lattice vectors of the fundamental cell, which can be written as $\boldsymbol{Q} \equiv \frac{2\pi}{L}(n_1, n_2, \cdots, n_d)$ when the fundamental cell is a cube of side length $L$.

In the case of dispersions of identical nonoverlapping spheres of radius $a$, the spectral density (S2) can be simplified as [3]

$$\tilde{\chi}_{_V}(\boldsymbol{Q}) = \phi_2\, \tilde{\alpha}_2(Q;a)\, S(\boldsymbol{Q}), \tag{S3}$$

where $\phi_2$ is the packing fraction, $Q \equiv |\boldsymbol{Q}|$, $\tilde{\alpha}_2(Q;a) \equiv 2^d \pi^{d/2}\, \Gamma(1+d/2)\, [J_{d/2}(Qa)]^2/Q^d$, and the structure factor $S(\boldsymbol{Q})$ for particle centers can be computed from the following expression;

$$S(\boldsymbol{Q}) = \frac{1}{N}\left|\sum_{j=1}^{N} e^{-i\boldsymbol{Q}\cdot\boldsymbol{r}_j}\right|^2. \tag{S4}$$

Therefore, one can easily obtain stealthy hyperuniform and stealthy nonhyperuniform dispersions from the associated point patterns by circumscribing the points by identical nonoverlapping spheres. In the absence of long-range order, $S(\boldsymbol{Q})$ converges to 1 for large wavenumbers, which implies that

$$\tilde{\chi}_{_V}(\boldsymbol{Q}) \approx \phi_2\, \tilde{\alpha}_2(|\boldsymbol{Q}|;a), \qquad |\boldsymbol{Q}| \to \infty. \tag{S5}$$

## II. KNOWN CLOSED-FORM EXPRESSIONS FOR PAIR STATISTICS

Here we summarize analytical expressions that we have used to evaluate the attenuation function $F(Q)$ for 3D overlapping spheres and 3D equilibrium hard spheres.

### A. Overlapping spheres

The autocovariance function is given by [1]:

$$\chi_V(r) = \exp\left(-\frac{4\pi}{3}a^3\rho\left\{2\,\Theta(r-2a) + \left[1+\frac{3r}{4a}-\frac{1}{16}\left(\frac{r}{a}\right)^3\right]\Theta(2a-r)\right\}\right) - \phi_2(\rho,a)^2, \tag{S6}$$

where the Heaviside step function is

$$\Theta(x) \equiv \begin{cases} 1, & x>0 \\ 0, & \text{otherwise}, \end{cases}$$

and the volume fraction of the dispersed phase is

$$\phi_2(\rho,a) = \exp\left(-\rho\frac{4\pi}{3}a^3\right), \tag{S7}$$

where $\rho$ is the number density of centers and $a$ is radius of decorated spheres.

### B. Equilibrium hard spheres

The spectral density of equilibrium hard spheres or, equivalently, equilibrium hard-sphere fluid is computed from Eq. (S3) using the structure factor $S(Q)$ in the Percus-Yevick approximation [1];

$$\begin{aligned} S(Q) = \Bigg(1 - \rho\frac{16\pi a^3}{q^6}\Big\{&[24a_1\phi_2 - 12(a_1+2a_2)\phi_2 q^2 + (12a_2\phi_2 + 2a_1 + a_2\phi_2)q^4]\cos(q) \\ &+ [24a_1\phi_2 q - 2(a_1 + 2a_1\phi_2 + 12a_2\phi_2)q^3]\sin(q) - 24\phi_2(a_1 - a_2q^2)\Big\}\Bigg)^{-1}, \end{aligned} \tag{S8}$$

where $a$ is radius of nonoverlapping spheres, $q = 2Qa$, $a_1 = (1+2\phi_2)^2/(1-\phi_2)^4$, and $a_2 = -(1+0.5\phi_2)^2/(1-\phi_2)^4$.

## III. GENERATION OF STEALTHY HYPERUNIFORM/NONHYPERUNIFORM DISPERSIONS

We explain how to generate stealthy hyperuniform/nonhyperuniform dispersions numerically. We first generate stealthy point configurations consisting of $N$ particles in a fundamental cell under periodic boundary conditions via the collective-coordinate optimization technique [4–6], which amounts to finding numerically the ground-state configurations for the following potential energy;

$$\Phi(\boldsymbol{r}^N) = \frac{1}{V_{\mathcal{F}}}\sum_{\boldsymbol{Q}}\tilde{v}(\boldsymbol{Q})\,S(\boldsymbol{Q}) + \sum_{i<j}u(r_{ij}), \tag{S9}$$

where

$$\tilde{v}(\boldsymbol{Q}) = \begin{cases} 1, & Q_{\text{lower}} < |\boldsymbol{Q}| \le Q_{\text{upper}} \\ 0, & \text{otherwise} \end{cases}, \tag{S10}$$

and a soft-core repulsive term [7]

$$u(r) = \begin{cases} (1-r/\sigma)^2, & r<\sigma \\ 0, & \text{otherwise} \end{cases}. \tag{S11}$$

We note that different from usual collective-coordinate procedures [4–6], the interaction (S9) used in this work includes a soft-core repulsive energy (S11) employed in Ref. [7]. Thus, the associated ground-state configurations are stealthy [i.e., $S(\boldsymbol{Q}) = 0$ for $Q_{\text{lower}} < |\boldsymbol{Q}| < Q_{\text{upper}}$], and their interparticle distances are larger than the length scale $\sigma$ due to the soft-core repulsions $u(r)$. The resulting point configurations are stealthy hyperuniform if $Q_{\text{lower}} = 0$ but otherwise stealthy nonhyperuniform. We then circumscribe the points by identical nonoverlapping spheres of radius $a < \sigma/2$.

We list parameters used to generate the disordered stealthy hyperuniform and disordered stealthy nonhyperuniform dispersions in Table. **??**.

TABLE S1. Parameters for disordered stealthy hyperuniform and disordered stealthy nonhyperuniform dispersions in $\mathbb{R}^3$.

| Parameters | Stealthy hyperuniform | Stealthy nonhyperuniform |
|---|---|---|
| Particle number $N$ | 1000 | 1000 |
| $\rho$ | 1 | 1 |
| The number of configurations | 300 | 300 |
| $(Q_{\text{lower}}a, Q_{\text{upper}}a)$ | (0, 1.5) | (1.0, 1.5) |
| $\sigma$ | 0.8 | 0.8 |
| $a$ | 0.3908 | 0.3908 |

## IV. ATTENUATION FUNCTION

In this section, we discuss how we derive the attenuation function $F(Q)$ from $\mathcal{F}(Q)$ in order to extend the range of applicable wavelengths of the original strong-contrast approximation derived by Rechtsman and Torquato [8]. We then explain how to compute $F(Q)$ numerically from the spectral density $\tilde{\chi}_{_V}(\boldsymbol{Q})$ of two-phase media. For statistically isotropic two-phase two-phase media in $\mathbb{R}^d$, the microstructure-dependent parameter $\mathcal{F}(Q)$ [see also Eq. (16) in the main text] that was employed in the original dynamic strong-contrast approximation for the effective dielectric constant $\epsilon_e(k_1)$ [8] is given as

$$\mathcal{F}(Q) \equiv -\frac{2^{d/2}\,\Gamma(d/2)}{\pi} Q^2 \int \frac{i}{4}\left(\frac{Q}{2\pi r}\right)^{d/2-1} H^{(1)}_{d/2-1}(Qr)\,\chi_{_V}(r)\,\mathrm{d}\boldsymbol{r}\,, \tag{S12}$$

where $\Gamma(x)$ is the gamma function, and $H^{(1)}_\nu(x)$ is the Hankel function of the first kind and order $\nu$. One can simplify the imaginary part of Eq. (S12) by using the definitions of $H^{(1)}_\nu(x)$ and the spherical Fourier transform in $\mathbb{R}^d$:

$$\mathrm{Im}[\mathcal{F}(Q)] = -Q^d\,\tilde{\chi}_{_V}(Q)\,/(2\pi)^{d/2}. \tag{S13}$$

Substituting this imaginary part into the original strong-contrast approximation [8] yields $\mathrm{Im}[\epsilon_e(k_1)\,/\epsilon_1] \propto \mathrm{Im}[\mathcal{F}(k_1)] = -{k_1}^d\,\tilde{\chi}_{_V}(k_1)\,/(2\pi)^{d/2}$ which quantifies the degree of attenuation for the electromagnetic waves in the media because $\gamma_e(k_1) = \mathrm{Im}\left[\sqrt{\epsilon_1/\,\epsilon_e(k_1)}\right]$. This implies that the original approximation does not fully account for attenuation due to scattering because the term $\tilde{\chi}_{_V}(Q = k_1)$ corresponds to the scattering intensity only at a single scattering angle $\theta = \pi/3$ such that $k_1 = 2k_1\sin(\theta/2)$; see also Sec. I. Consequently, while the original approximation [8] still can provide an accurate estimate of $\epsilon_e(k_1)$ in the long-wavelength regime ($k_1\ell \ll 1$), it is strictly not valid in the intermediate-wavelength regime ($k_1\ell \sim 1$).

In order to extend the range of applicable wavelengths of the original strong-contrast approximation [8], we modify $\mathcal{F}(Q)$ to account for the contribution from spatial variation of the sinusoidal incident waves, e.g., $\exp(ik_1x)$. The modified microstructure-dependent parameter is the *attenuation function* $F(Q)$, defined by the following integral:

$$F(Q) = -\frac{2^{d/2}\,\Gamma(d/2)}{\pi} Q^2 \int \frac{i}{4}\left(\frac{Q}{2\pi r}\right)^{d/2-1} H^{(1)}_{d/2-1}(Qr)\,e^{-iQ\hat{\boldsymbol{k}}\cdot\boldsymbol{r}}\,\chi_{_V}(\boldsymbol{r})\,\mathrm{d}\boldsymbol{r} \tag{S14}$$

$$= -\frac{2^d\,\Gamma(d/2)}{\pi^{1-d/2}} Q^2 \int_0^\infty r^{d-1}\frac{J_{d/2-1}(Qr)}{(Qr)^{d/2-1}}\frac{i}{4}\left(\frac{Q}{2\pi r}\right)^{d/2-1} H^{(1)}_{d/2-1}(Qr)\,\chi_{_V}(r)\,\mathrm{d}r\,, \tag{S15}$$

where $J_\nu(x)$ is the Bessel function of the first kind and order $\nu$, and $\hat{\boldsymbol{k}}$ is the unit wavevector in the direction of the incident waves. The expression (S14), identical to Eq. (18) in the main text, can be simplified as Eq. (S15) because the autocovariance function is radial due to the statistical isotropy. Note that the factor $\exp\left(-iQ\hat{\boldsymbol{k}}\cdot\boldsymbol{r}\right)$ in the integrand of Eq. (S14) represents the incident waves.

Now we discuss how to compute $F(Q)$ numerically. In three dimensions, the imaginary and real parts of Eq. (S15) can be simplified as follows: in the direct space representation,

$$\mathrm{Im}[F(Q)] = -\sqrt{\frac{\pi}{2}} Q^2 \int_0^\infty r\,J_{1/2}(Qr)^2\,\chi_{_V}(r)\,\mathrm{d}r\,, \tag{S16}$$

$$\mathrm{Re}[F(Q)] = \sqrt{\frac{\pi}{2}} Q^2 \int_0^\infty r\,J_{1/2}(Qr)\,Y_{1/2}(Qr)\,\chi_{_V}(r)\,\mathrm{d}r\,, \tag{S17}$$

where $Y_\nu(x)$ is the Bessel function of the second kind and order $\nu$. The same quantities also can be evaluated in the Fourier space representation:

$$\mathrm{Im}[F(Q)] = -\frac{Q}{2(2\pi)^{3/2}} \int_0^{2Q} q\, \tilde{\chi}_{_V}(q)\, \mathrm{d}q\,, \tag{S18}$$

$$\mathrm{Re}[F(Q)] = -\frac{2Q^2}{\pi} \mathrm{p.v.} \int_0^{\infty} \mathrm{d}q\, \frac{1}{q(Q^2-q^2)}\, \mathrm{Im}[F(q)], \tag{S19}$$

where p.v. stands for the Cauchy principal value. While Eqs. (S16)-(S17) and Eqs. (S18)-(S19) are equivalent, accurate numerical estimation of the former is generally more challenging because it is numerically and experimentally difficult to ascertain accurately the large-$r$ tail of the autocovariance function $\chi_{_V}(r)$ for disordered media. On the other hand, the large-$Q$ (i.e., short wavelength) behavior of $\tilde{\chi}_{_V}(Q)$, required for Eq. (S19), can be easily obtained from Eq. (S5). Thus, we mainly use the Fourier representations (S18) and (S19) in this study. In practice, Eq. (S19) can be computed numerically with an upper limit $M$ as follows:

$$\mathrm{Re}[F(Q)] \approx -\frac{2Q^2}{\pi} \mathrm{p.v.} \int_0^{M} \frac{1}{q(Q^2-q^2)}\, \mathrm{Im}[F(q)]\, \mathrm{d}q \tag{S20}$$

$$= -\frac{2}{\pi} Q \left[ \int_0^M \frac{\mathrm{Im}[F(q)]}{(Q+q)q}\, \mathrm{d}q + \int_0^M \frac{\mathrm{Im}[F(q)] - \mathrm{Im}[F(Q)]}{Q^2-q^2}\, \mathrm{d}q + \frac{\mathrm{Im}[F(Q)]}{2Q} \ln\left|\frac{M+Q}{M-Q}\right| \right]. \tag{S21}$$

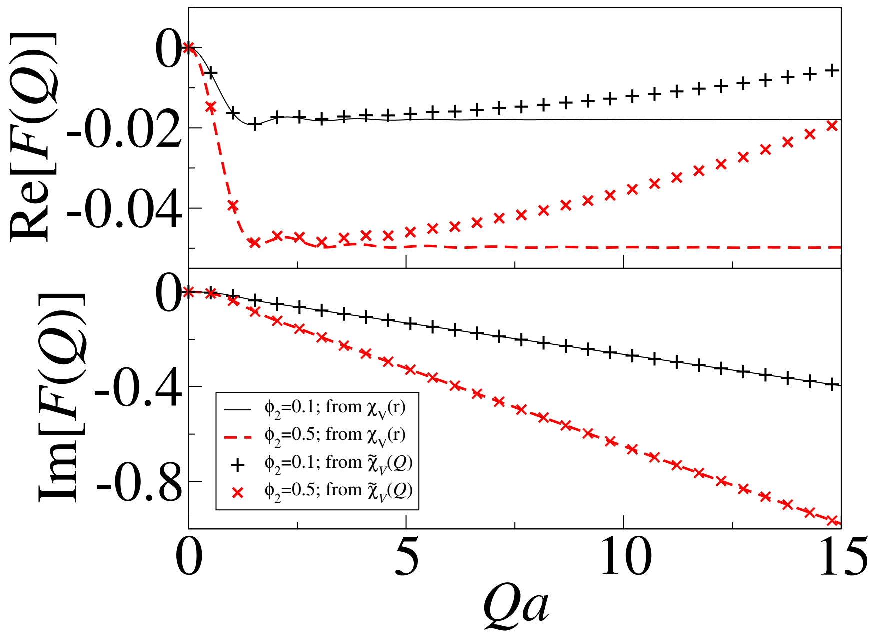


FIG. S1. Evaluation of the attenuation function $F(Q)$ for 3D overlapping spheres with $\phi_2 = 0.1, 0.5$ using two different methods: numerical integrals over $\chi_{_V}(r)$, denoted by "from $\chi_{_V}(r)$" [see Eqs. (S16) and (S17)], and numerical integrals over $\tilde{\chi}_{_V}(Q)$, denoted by "from $\tilde{\chi}_{_V}(Q)$" [Eq. (S18) and Eq. (S21) with $M = 300$]. Results from these two methods show excellent agreement at small wavenumbers $Qa < 5$. Therefore, we can use the approximation (S21) at small wavenumbers, which is easier to compute numerically in practice.

For purposes of illustration, we compute the attenuation function of 3D overlapping spheres via two different representations [Eqs. (S16) and (S17)] and [Eqs. (S18) and (S21)] and compare them in Fig. S1. Since the autocovariance function $\chi_{_V}(\boldsymbol{r})$ of 3D overlapping spheres has compact support, the integrals (S16) and (S17) in direct space can be accurately computed. In Fig. S1, we clearly see that that the imaginary parts $\mathrm{Im}[F(Q)]$ obtained from Eqs. (S16) and (S18) are identical. For the real part $\mathrm{Re}[F(Q)]$, the estimate from Eq. (S21) provides a reasonable approximation of Eq. (S17) up to intermediate wavenumbers ($Qa < 5$). Thus, we use the approximation (S21) in the present study where we investigate the effective properties down to the intermediate-wavelength regime.

## V. COMPARISON OF MICROSTRUCTURE-DEPENDENT STRONG-CONTRAST AND OTHER APPROXIMATIONS

We compare the modified microstructure-dependent strong-contrast approximations [i.e., Eqs. (4), (8), and (9) in the main text] with other commonly employed approximations for both the effective dynamic dielectric constant and elastic moduli. We focus on 3D stealthy hyperuniform dispersions and simple cubic lattice dispersions of identical spheres of radius $a$. These examples will provide stringent tests of the predictive power of the various approximations at finite wavenumbers because they exhibit nontrivial spatial correlations at intermediate length scales, which are not typical of most amorphous systems. We will see that the strong-contrast approximations are far superior in predicting the effective properties in the intermediate-wavelength regime when compared to the corresponding predictions of all of these other estimates.

To test the validity and predictive capability of our microstructure-dependent formulas for the effective dynamic properties via numerical simulations, we devised the first dynamic extensions of the fast-Fourier transformation homogenization schemes by Moulinec and Suquet (1998) and Eyre and Milton (1999) [9, 10] for the purely static problems. In 3D, we carry out simulations for spheres distributed in a matrix on the sites of a simple cubic lattice, which importantly are stealthy, even if ordered. These idealized periodic model microstructures served several purposes:

- They provide stringent tests of any approximate formula because such systems are dissipationless ($\mathrm{Im}[\epsilon_e(k_1)] = 0$ or $\mathrm{Im}[K_e(k_{L_1})] = 0$) up to a finite wavenumber because they suppress scattering down to such intermediate wavelengths. Moreover, the real parts of $\epsilon_e(k_1)$ or $K_e(k_{L_1})$ must exhibit sharp transitions for $\lambda/2 \sim$ lattice constant due to Bragg diffraction, which arises from the constructive interference of all waves scattered by such periodic structures.
- Disordered stealthy hyperuniform dispersions are expected to share the same dissipationless properties as the simple cubic dispersion, in sharp contrast to garden-variety disordered media, and hence lessons learned about the predictive power of our approximations from the periodic examples are expected to extend to these exotic amorphous materials.
- Numerical study of simple periodic microstructure enables us to use a very fine grid resolution.

Using our numerical code, we managed to obtain some results for simple cubic dispersions for certain contrast ratios, as reported below. Estimates based on the simulations and our modified strong-contrast approximations show excellent agreement for simple cubic dispersions, including the sharp transition due to Bragg diffraction. We show that conventional formulas for effective dynamic properties fail to predict such sharp transitions.

We attempted to apply our code when the fundamental unit cell contained multiple particles, as would be the case for any disordered composite. However, we could not overcome numerical convergence issues in such situations to make any definitive conclusions. Nonetheless, we still endeavored to test the predictions of our formulas that disordered stealthy hyperuniform composites should be dissipationless (as described above) by carrying numerical simulations. To do so, we use a publicly available finite-difference frequency-domain method code [11] to compute the wavenumber-dependent effective dielectric constant of 2D disordered stealthy hyperuniform dispersions at a packing fraction of 0.25. The results of these numerical studies indeed confirmed our expectations of the high accuracy of our 2D formulas for a wide range of wavenumbers when the contrast ratio was less than 10. Since this property is independent of the space dimension, it will also apply to 3D stealthy media. Importantly, we also confirmed that standard disordered dispersions are not dissipationless.

In summary, all of these simulation results imply that our approximations can provide accurate estimates of the effective dynamic properties down to the intermediate-wavelength regime and hence are superior to conventional approximations. Specific details are provided below.

### A. Dynamic dielectric constants

We compute the effective dynamic dielectric constants of two-phase composite materials from the microstructure-dependent strong-contrast (an extended version of the formula given in Ref. [8]), Maxwell-Garnett [12, 13], and quasicrystalline approximations [12]. For simple cubic lattice dispersions, we compare these estimates with numerical simulations based on the fast-Fourier transform homogenization schemes [9, 10].

The explicit formula of the strong-contrast approximation (4) in the main text can be rewritten as

$$\beta {\phi_2}^2 \left[\frac{\epsilon_e(k_1) - \epsilon_1}{\epsilon_e(k_1) + 2\epsilon_1}\right]^{-1} = \phi_2 - A_2(k_1)\,\beta, \tag{S22}$$

where $k_1$ is the wavenumber of electromagnetic waves in the reference phase (phase 1) and $\beta \equiv (\epsilon_2 - \epsilon_1)/(\epsilon_2 + 2\epsilon_1)$ is the dielectric polarizabilitiy. Note that the modified formula of $A_2(Q)$ [see Eq. (5) in the main text] is different from the original

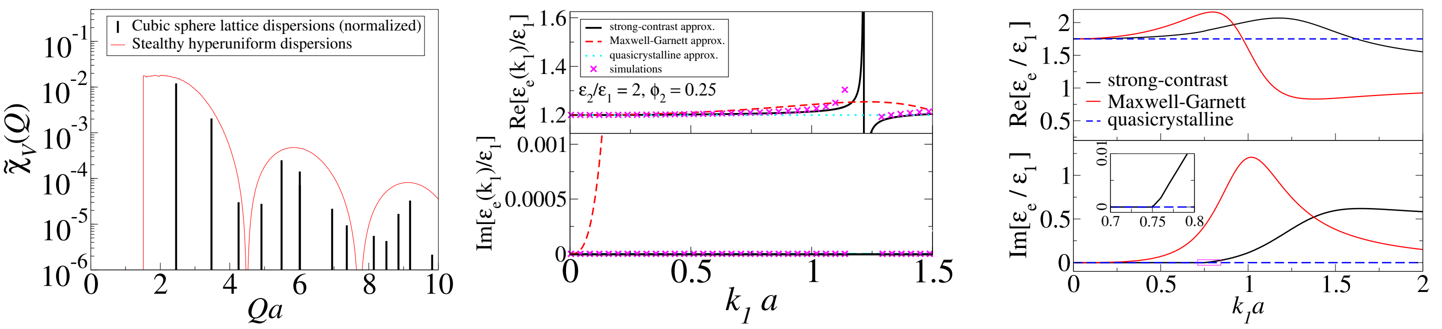


(a) (b) (c)

FIG. S2. Evaluation of the spectral density and the effective dynamic dielectric constant for simple cubic lattice dispersions and 3D "disordered" stealthy hyperuniform dispersions of identical nonoverlapping spheres of radius $a$ and $\phi_2 = 0.25$. (a) The spectral densities of two stealthy hyperuniform dispersions. For purposes of illustration, the heights of the Bragg peaks are normalized by the particle number. (b) The effective dielectric constant $\epsilon_e(k_1)$ of simple cubic lattice dispersions of $\epsilon_2/\epsilon_1 = 2$. Note that the strong-contrast approximation (S22) captures that the real part Re[$\epsilon_e$] has a sharp transition around $k_1 a \approx 1.227$ due to the Bragg diffraction, but the imaginary part Im[$\epsilon$] is zero except around $k_1 a \approx 1.227$, which, unlike the Maxwell-Garnett approximation, is consistent with the numerical simulations. (c) The effective dielectric constant of 3D disordered stealthy hyperuniform dispersions of $\epsilon_2/\epsilon_1 = 13$. The inset in the lower panel is a magnification around $k_1 a = 0.75$, which clearly demonstrates that the strong-contrast approximation correctly predicts the transparency regime for the stealthy hyperuniform dispersions, but the others cannot.

expression given in Ref. [8] in that the former accounts for the spatial variation of the incident waves, but the latter does not; see *Materials and Methods* in the main text and Sec. IV.

We also consider the Maxwell-Garnett approximation that are derived by substituting the dielectric polarizability of a single dielectric sphere into the Clausius-Mossotti equation, which consequently ignores the spatial correlations of particles [13]:

$$\phi_2{}^2 \beta \left[\frac{\epsilon_e(k_1) - \epsilon_1}{\epsilon_e(k_1) + 2\epsilon_1}\right]^{-1} = \phi_2 - (1-\phi_2)\phi_2 \left[(k_1 a)^2 + i\frac{2}{3}(k_1 a)^3\right]\beta. \tag{S23}$$

Hence, this formula is only valid for very low packing fractions of a few percent [14].

The quasicrystalline approximation estimates the effective dynamic dielectric constant $\epsilon_e(k_1)$ by using the "effective" Green's function of many-body systems (dispersions) up to the level of pair correlation function $g_2(\boldsymbol{r})$ [15]. However, this is done in such a way that it only accounts for the structure factor in the infinite-wavelength limit [15] [i.e., $S(0) = 1 + \rho \int (g_2(\boldsymbol{r}) - 1)\,\mathrm{d}\boldsymbol{r}$] and consequently, the spatial correlations at finite wavelengths are ignored. In the low-concentration limit, the quasicrystalline approximation can be explicitly written as follows [12]:

$$\phi_2{}^2 \beta \left[\frac{\epsilon_e(k_1) - \epsilon_1}{\epsilon_e(k_1) + 2\epsilon_1}\right]^{-1} = \phi_2 + i\left\{\frac{2}{3}\phi_2\, S(0)\,(k_1 a)^3 \left[1 - i\frac{2}{3(1-\beta\phi_2)}(k_1 a)^3\, S(0)\right]^{-1}\right\}\beta. \tag{S24}$$

Comparing the right-hand sides of Eqs. (S22)-(S24) reveals that the sign convention of the imaginary part Im[$\epsilon_e$] of Eq. (S24) is different from others.

Stealthy hyperuniform dispersions and simple cubic lattice dispersions are models that provide stringent tests of the predictive power of the various approximations for the aforementioned reasons. For these two stealthy hyperuniform systems of $\phi_2 = 0.25$ [i.e., $\tilde{\chi}_V(Q) = 0$ in a region around the origin as shown in Fig. S2a], we compare those three aforementioned approximations in Fig. S2 (b) and (c). The Maxwell-Garnett (S23) and quasicrystalline (S24) approximations are formally similar to the strong-contrast approximation, and these three approximations give identical results in the static limit. At finite wavelengths, however, estimates from these three approximations are considerably different. For simple cubic lattice dispersions (Fig. S2b), the strong-contrast approximation [where $F(Q)$ is computed from Eq. (19) in the main text] successfully captures the transition in Re[$\epsilon_e(k_1)$] due to the Bragg diffraction. The strong-contrast approximation also predicts that the simple cubic structure is transparent [i.e., Im[$\epsilon_e(k_1)$] = 0] due to its stealthy hyperuniformity down to a finite wavelength but exhibits strong-attenuation (not depicted in the figure) when the Bragg diffraction condition is satisfied. Importantly, these results are consistently observed in the numerical simulations. However, the other approximations fail to predict Bragg diffraction. The high predictive power of the strong-contrast approximation is due to the fact that the contributions from

the spatial correlations of the composites at the finite wavelengths are included, which the other approximations neglect. Furthermore, this example vividly demonstrates that the strong-contrast approximation can provide a reasonable estimate of $\epsilon_e$ at the wavelengths comparable to the interparticle distance, where ordinary homogenization theories are generally no longer valid.

For 3D stealthy hyperuniform dispersions, our strong-contrast approximation predicts that they are transparent ($\mathrm{Im}[\epsilon_e] = 0$) up to a finite wavenumber ($k_1 a < Q_{\mathrm{upper}} a/2$); see the lower panel of Fig. S2(c). This prediction is consistent with a previous different study by Leseur *et al.* [16], which demonstrated that the stealthy hyperuniform dispersions are transparent at finite wavenumbers even in the optically dense regime. By contrast, the Maxwell-Garnett estimate cannot capture the transparency of stealthy hyperuniform dispersions because this phenomenon results from the spatial correlations in the stealthy hyperuniform dispersions, but the Maxwell-Garnett ignore the spatial correlations at any length scales. The quasicrystalline approximation accounts for the spatial correlations of composites only in the long-wavelength regime (i.e., $k_1 = 0$), leading to a wavenumber-independent dispersion relation. Thus, it cannot capture the fact that the stealthy hyperuniform dispersions are no longer transparent when $k_1 > Q_{\mathrm{upper}}/2$.

### B. Dynamic elastic moduli

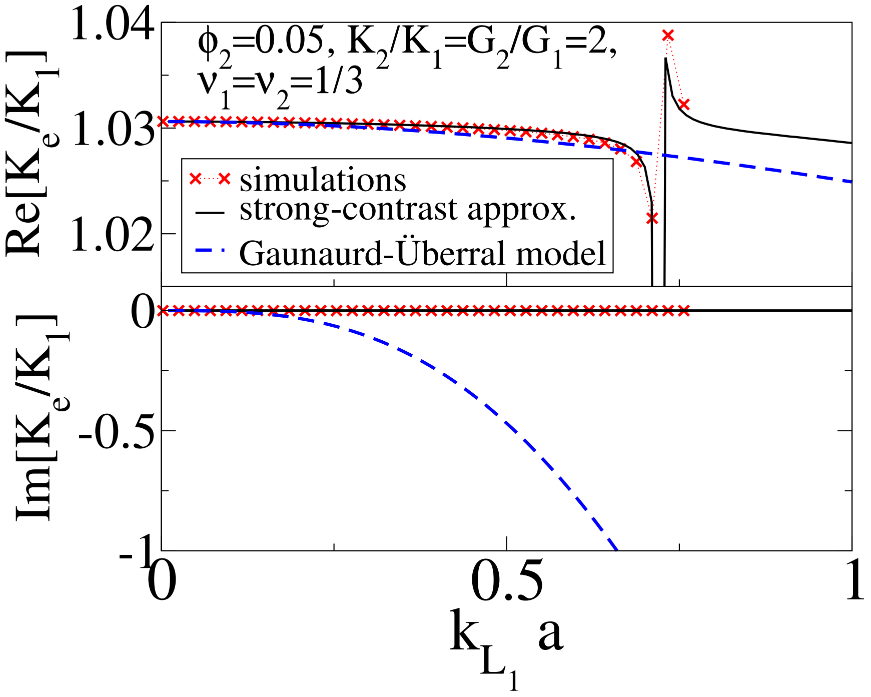


FIG. S3. Evaluation of the effective bulk modulus $K_e$ for simple cubic lattice dispersions of identical spheres of radius $a$, $\phi_2 = 0.05$, $K_2/K_1 = G_2/G_1 = 2$, and $\nu_1 = \nu_2 = 1/3$. Here, $k_{L_1}$ is the longitudinal wavenumber in phase 1. The strong-contrast approximation (S25) can capture a sharp transition in $\mathrm{Re}[K_e]$ due to the Bragg diffraction and the transparency (i.e., $\mathrm{Im}[K_e] = 0$) due to stealthy hyperuniformity. These results are consistent with the numerical simulations. By contrast, the Gaunaurd-Überall model (S29) fails to predict the sharp transition in the real part and the transparency for most wavenumbers up to the Bragg condition.

We compare the effective dynamic elastic moduli of two-phase composites from the modified microstructure-dependent strong-contrast approximations [Eqs. (8) and (9) in the main text] and the Gaunaurd-Überall model [17], which is very similar in spirit to the Maxwell-Garnett expression for the dielectric situation. In three dimensions, the strong-contrast

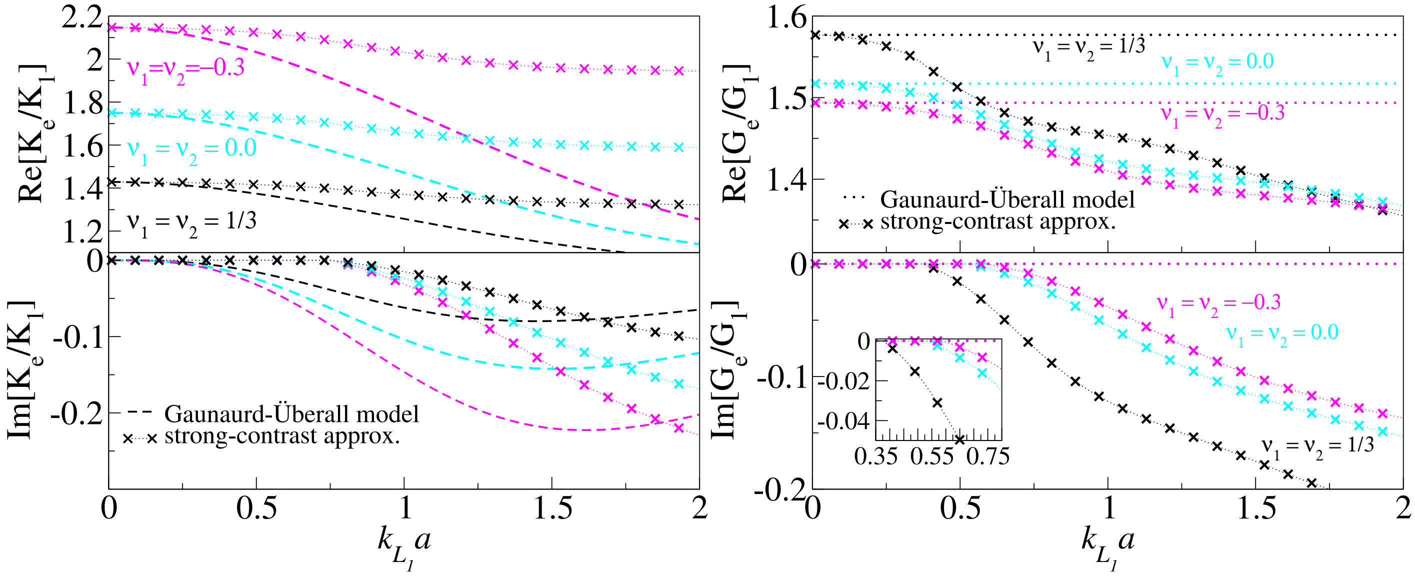


(a) (b)

FIG. S4. Evaluation of the effective bulk modulus $K_e$ (a) and effective shear modulus $G_e$ (b) for 3D stealthy hyperuniform dispersions of identical spheres of radius $a$ and $\phi_2 = 0.25$ as predicted by the strong-contrast approximations (S25)-(S26) and the Gaunaurd-Überall model (S29)-(S30). Here, the contrast ratios of the particle (phase 2) to the matrix (phase 1) phases are $K_2/K_1 = G_2/G_1 = 13$, and $k_{L_1}$ is the longitudinal wavenumber in the matrix phase. The effective elastic moduli are computed at three different values of Poisson ratios ($\nu_1 = \nu_2 = 1/3, 0, -0.3$). These two approximations give the identical results in the static case ($k_{L_1} = 0$) but yield considerably different results at the intermediate wavenumbers ($0 < k_{L_1} a < 2$). This discrepancy arises because the strong-contrast approximations account for the spatial correlations at the short/intermediate length scales, which are neglected in the Gaunaurd-Überall model.

approximations (8) and (9) in the main text can be rewritten as

$$\frac{K_e(k_{L_1}) - K_1}{K_e(k_{L_1}) + 4G_1/3} = \frac{{\phi_2}^2 \kappa}{\phi_2 - C_2(k_{L_1})}, \tag{S25}$$

$$\frac{G_e(k_{L_1}) - G_1}{G_e(k_{L_1}) + \frac{[3K_1/2+4G_1/3]G_1}{K_1+2G_1}} = \frac{{\phi_2}^2 \mu}{\phi_2 - D_2(k_{L_1})}, \tag{S26}$$

where $C_2$ and $D_2$ are functionals involving the attenuation function [see Eqs. (10) and (11) in the main text], and

$$\kappa = \frac{K_2 - K_1}{K_2 + 4G_1/3}, \tag{S27}$$

$$\mu = \frac{G_2 - G_1}{G_2 + [3K_1/2 + 4G_1/3]\, G_1/(K_1 + 2G_1)}, \tag{S28}$$

are the polarizabilities for bulk and shear moduli, respectively.

The Gaunaurd-Überall model estimates the effective dynamic elastic moduli for dispersions of spherical particles in the low-frequency regime. Since this model accounts solely for the scattering due to a single particle, it can be regarded as the elastodynamic counterpart of the Maxwell-Garnett approximation. We use the expressions taken from Ref. [17]:

$$\frac{K_e(k_{L_1}) - K_1}{K_e(k_{L_1}) + 4G_1/3 - [\Gamma_e R^2 (k_{L_1} a)^2 - iR^3 (k_{L_1} a)^3 (K_e(k_{L_1}) - K_1)]/3} = \frac{\phi_2 \kappa}{1 - [\Gamma_2 (k_{L_1} a)^2/(3K_2 + 4G_1) - i(k_{L_1} a)^3 \kappa/3]}, \tag{S29}$$

$$\frac{G_e(k_{L_1}) - G_1}{G_e(k_{L_1}) + \frac{[3K_1/2+4G_1/3]G_1}{K_1+2G_1}} = \phi_2 \mu, \tag{S30}$$

where $\rho_e = \rho_1 + \phi_2(\rho_2 - \rho_1)$, $R$ represents the radius of a specimen, which is often set to be zero [17], and $\Gamma_i$ (for $i = 2, e$) are given as

$$\Gamma_i = K_1 - \frac{3}{2}K_i - \frac{2}{3}G_1 + \frac{\rho_i}{2\rho_1}\frac{3K_1+4G_1}{3K_i+4G_i}\left[K_i + \frac{4}{5}(G_1 + \frac{2}{3}G_i)\right]. \tag{S31}$$

Now we compare the strong-contrast approximations (S25)-(S26) with the Gaunaurd-Überall approximations (S29)-(S30) for simple cubic lattice dispersions ($\phi_2 = 0.05$) and 3D stealthy hyperuniform dispersions ($\phi_2 = 0.25$), since these systems will serve as severe test of the approximations. We consider the simple cubic lattice dispersions of $\phi_2 = 0.05$, $K_2/K_1 = G_2/G_1 = 2$, and $\nu_1 = \nu_2 = 1/3$. Figure S3 compares the effective bulk modulus evaluated from the aforementioned formulas as well as the numerical simulations based on the fast-Fourier transformation homogenization schemes [9, 10]. The numerical simulations are carried out in the presence of the longitudinal applied strain field, i.e., $\epsilon_{\mathbf{0}}(\mathbf{r}) = \hat{\boldsymbol{x}}\hat{\boldsymbol{x}}\exp(i\,k_{L_1}\hat{\boldsymbol{x}}\cdot\boldsymbol{r})$, where $\hat{\boldsymbol{x}}$ is the unit vector in $+x$ direction. The strong-contrast approximation and simulation results show excellent agreement with one another. Both correctly capture the sharp transition in $\mathrm{Re}[K_e]$ as a function of wavenumber due to Bragg diffraction and the transparency (i.e., $\mathrm{Im}[K_e] = 0$) due to the stealthy hyperuniformity of a lattice dispersion. By contrast, the Gaunaurd-Überall formulas cannot capture such salient physics because they ignore the spatial correlations at any length scale.

We compare the estimates of $K_e$ and $G_e$ from the aforementioned two formulas for 3D disordered stealthy hyperuniform dispersions. Figure S4 presents the results for $\phi_2 = 0.25$, $K_2/K_1 = G_2/G_1 = 13$, and $\rho_1 = \rho_2$ at three different values of the Poisson ratios $\nu_1(= \nu_2) = 1/3, 0$, and $-0.3$. In the static limit, these two approximations yield identical results for both the effective bulk and shear moduli. At finite wavenumbers ($0 < k_{L_1}a < 2$), however, the strong-contrast approximation captures that the effective bulk moduli becomes lossless (i.e., $\mathrm{Im}[K_e] = 0$) up to $k_{L_1}a = 0.75$, which the estimate (S29) cannot predict. For the effective shear moduli, we note that the approximation (S30) is independent of the wavenumber. However, the strong-contrast approximation predicts that the effective shear modulus becomes lossless at long wavelengths, which correspond to the cases where the "transverse wavenumber" is half of the exclusion radius, i.e., $k_{T_1}a < 0.75$. Such striking differences between these two approximations at finite wavenumbers result from the fact that the strong-contrast approximations account for the spatial correlations in composites, but the Gaunaurd-Überall approximations do not.

## VI. THE EFFECTIVE DYNAMIC ELASTIC MODULI OF DISPERSIONS OF SPHERICAL CAVITIES

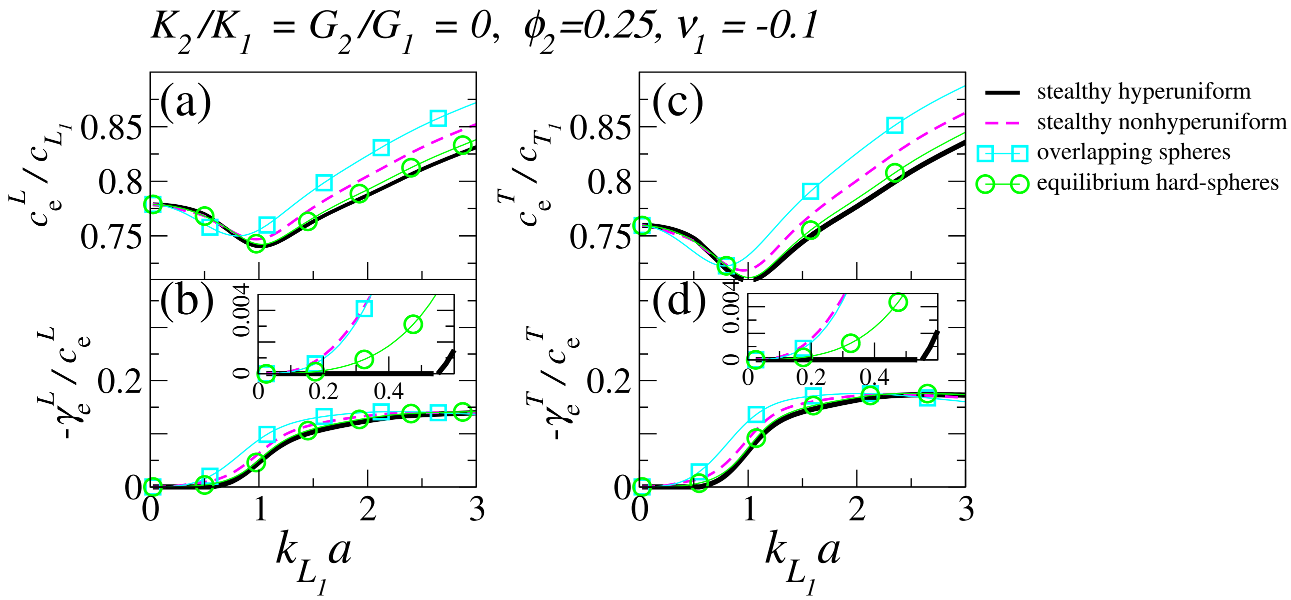


FIG. S5. Estimates of scaled effective elastic wave characteristics for 3D dispersions of spherical cavities of radius $a$ in a compressible matrix phase with Poisson ratio $\nu_1 = -0.1$ (i.e., $K_2/K_1 = G_2/G_1 = 0$) by the strong-contrast approximations (S25) and (S26). Here, $k_{L_1}$ is the wavenumber of longitudinal waves in phase 1, and $c_{L_1}$ and $c_{T_1}$ are wave speeds of longitudinal and transverse waves, respectively, in phase 1. (a,c) Effective wave speeds and (b,d) effective attenuation coefficients are plotted in terms of $k_{L_1}a$. For stealthy hyperuniform dispersions, $\gamma_e^{L,T} = 0$ when $k_{L_1}a \lesssim 0.55$.

We estimate the scaled effective wave propagation properties of the four different models of 3D dispersions. As noted in the main text, we consider two special cases of phase moduli; $K_2/K_1 = G_2/G_1 = \infty$ and $\nu_1 = 1/3$ (i.e., $\kappa = 1$ and $\mu = 1$) and $K_2/K_1 = G_2/G_1 = 0$ and $\nu_1 = -0.1$ (i.e., $\kappa = -3/8$ and $\mu = -6/5$), where $\kappa$ and $\mu$ are the bulk and shear moduli "polarizabilities," respectively. The former case is presented in Fig. 3 in the main text, but we present the latter case here; see Fig. S5.

For each case of these prescribed phase properties, four different models have similar effective wave speeds but exhibit significantly different attenuation coefficients at small wavenumbers $k_{_{L_1}} a < 2$, i.e., the wavelength of the incident waves is larger than the particle diameter. Compared with the dispersions with rigid inclusions, the wave speeds are slower than those in phase 1 and barely change with $k_{_{L_1}} a$, leading to relatively flat profiles for the attenuation coefficients; see Fig. S5. In striking contrast to the other models, stealthy hyperuniform dispersions become lossless (i.e., $\gamma_e^{L,T} = 0$) for elastic waves for $k_{_{L_1}} a \lesssim 0.55$, which is predicted from Eq. (13) in the main text.

## VII. MATHEMATICAL PROPERTIES OF THE STRONG-CONTRAST EXPANSIONS

We briefly discuss two important mathematical properties of the strong-contrast expansions. We first discuss that they exhibit rapid convergence property even for high contrast ratios in Sec. VII A. We then discuss in Sec. VII B how truncation of these series leads to formulas that approximately and accurately account for microstructural information to all orders. In this section, for simplicity, we focus on the dynamic dielectric problems. However, we note that the ensuing discussions can be applied to strong-contrast expansions for electrostatic, elastostatic, and elastodynamic properties, and the modified strong-contrast approximations that we employed in the present work.

### A. Rapid convergence property

In order to understand the rapid convergence property of the strong-contrast expansions even for high contrast ratios, it is helpful to compare it with ordinary perturbation theories for the effective dielectric constant $\epsilon_e$ of composites, which is what we call the weak-contrast expansions. A formally exact weak-contrast expansion for $\epsilon_e(k_1)$ is a power series in terms of the simple difference between the dielectric constants of the reference (phase 1) and polarized (phase 2) phases as follows:

$$\frac{\epsilon_e(k_1)}{\epsilon_1} = 1 + \sum_{n=1}^{\infty} \mathcal{A}_n(k_1) \left(\frac{\epsilon_2 - \epsilon_1}{\epsilon_1}\right)^n, \tag{S32}$$

where $k_1$ is the wavenumber in phase 1 and $\mathcal{A}_n(k_1)$ is generally a functional of the $n$-point correlation function $S_n^{(i)}(\boldsymbol{x}_1, \cdots, \boldsymbol{x}_n)$ that we defined in the main text. Since Eq. (S32) is a power series in terms of the ratio $(\epsilon_2 - \epsilon_1)/\epsilon_1$, its convergence is guaranteed only when $\epsilon_1 \approx \epsilon_2$, which is the reason why perturbations of this type are called "weak-contrast" expansions.

By contrast, the formally exact strong-contrast expansion can be regarded as a power series in terms of the scalar polarizability $\beta$:

$$\frac{\epsilon_e(k_1)}{\epsilon_1} = 1 - \frac{d{\phi_2}^2\beta}{\phi_2(\phi_2\beta - 1) + \sum_{n=2}^{\infty} A_n \beta^{n-1}} \tag{S33}$$

where $A_n$ is a short-hand notation of the $k_1$-dependent functional $A_n(k_1) = A_n[S_1, \cdots, S_n]$ involving up to the $n$-point correlation functions. The series can be rewritten in the form of power series:

$$\begin{aligned}\frac{\epsilon_e(k_1)}{\epsilon_1} =& 1 + \underbrace{d\phi_2}_{B_1}\beta + \underbrace{d\left(A_2 + {\phi_2}^2\right)}_{B_2}\beta^2 + \underbrace{\frac{d}{\phi_2}\left({A_2}^2 + A_3\phi_2 + 2{\phi_2}^2 A_2 + {\phi_2}^4\right)}_{B_3}\beta^3 \\ &+ \underbrace{\frac{d}{{\phi_2}^2}\left({A_2}^3 + 2A_2A_3\phi_2 + 3{A_2}^2{\phi_2}^2 + A_4{\phi_2}^2 + 2A_3{\phi_2}^3 + 3A_2{\phi_2}^4 + {\phi_2}^6\right)}_{B_4}\beta^4 + \mathcal{O}(\beta^5),\end{aligned} \tag{S34}$$

where the $n$-th order coefficient $B_n$ is a functional of $A_2, \cdots, A_n$. It is important to note that the expansion parameter $\beta$ is always bounded as

$$-\frac{1}{d-1} \le \beta \equiv \frac{\epsilon_2 - \epsilon_1}{\epsilon_2 + (d-1)\epsilon_1} \le 1, \tag{S35}$$

and thus the radius of convergence of the exact series (S34) is much larger than that of the weak-contrast series (S32). In other words, Eq. (S34) can converge rapidly even for high contrast ratios.

### B. Accurate estimates by truncated expansions

It is important to note that the higher-order (functional) coefficients $B_n$ of the formally exact strong-contrast expansions can be approximated by lower-order (functional) coefficients $B_n^{(m)}$ of the expansions truncated at the $m$-point level. For this reason, the truncated expansions can provide accurate estimates of the formally exact expansions; see Eq. (S34). This property is attributed to the fact that the expansion (S33) is a rational function of $\beta$.

For instance, the microstructure-dependent approximation (S22) of $\epsilon_e(k_1)$ that is employed in this work is truncation of the series (S33) at the 2-point level. Thus, it can be rewritten as

$$\frac{\epsilon_e(k_1)}{\epsilon_1} \approx 1 + \frac{d\phi_2\beta}{1-(\phi_2 + A_2/\phi_2)\beta} \tag{S36}$$

$$= 1 + \underbrace{d\phi_2}_{B_1^{(2)}}\beta + \underbrace{d\left(A_2+{\phi_2}^2\right)}_{B_2^{(2)}}\beta^2 + \underbrace{\frac{d}{\phi_2}\left(A_2+{\phi_2}^2\right)^2}_{B_3^{(2)}}\beta^3 + \underbrace{\frac{d}{{\phi_2}^2}\left(A_2+{\phi_2}^2\right)^3}_{B_4^{(2)}}\beta^4 + \mathcal{O}(\beta^5), \tag{S37}$$

where the $n$th-order coefficient $B_n^{(2)} = B_n^{(2)}[A_2] \equiv d{\phi_2}^{2-n}(A_2+{\phi_2}^2)^{n-1}$ is a functional of $A_2$. Importantly, since $B_3 - B_3^{(1)} = dA_3$, this truncated series can well approximate the higher-order functionals of the exact series (S34) solely in terms of the single functional $A_2$ that involves with $\tilde{\chi}_V(Q)$.

In general, truncation of the strong-contrast expansion (S33) at the $m$-point level can be regarded as the Padé (rational) approximant of order (1,m) of the formally exact series (S34) of $\epsilon_e(k_1)$ in terms of a bounded parameter $\beta \in [-1/(d-1), 1]$. Such a truncated series can be rewritten as

$$\frac{\epsilon(k_1)}{\epsilon_1} \approx 1 - \frac{d{\phi_2}^2\beta}{\phi_2(\phi_2\beta-1)+\sum_{n=2}^m A_n\beta^{n-1}}$$
$$= 1 + d\phi_2\beta + B_2^{(m)}[A_2]\beta^2 + \cdots + B_m^{(m)}[A_2,\cdots,A_m]\beta^m + B_{m+1}^{(m)}[A_2,\cdots,A_m]\beta^{m+1} + \cdots, \tag{S38}$$

where the $n$th-order coefficient $B_n^{(m)}$ of this approximant is a functional of $A_2, \cdots, A_m$ and thus $B_n^{(m)}$ is identical to the $n$th order coefficient $B_n$ in the exact series (S34) for $n \le m$. Importantly, even for $n > m$, the $n$th order functionals $B_n^{(m)}$ in the truncated series can well approximate those in the formally exact series with a finite number of terms $A_2, \cdots, A_m$. Thus, truncating strong-contrast expansions at the $m$-point level can provide excellent approximations of the effective properties.

## VIII. CROSS-PROPERTY RELATIONS BETWEEN $\epsilon_e$ AND $K_e$

We present plots depicting cross-property relations for some other phase properties beyond the ones described in Fig. 4 in main text; see Figs. S6 and S7. We note that contours vary with phase properties $\epsilon_p$, $K_p$, $G_p$ for $p = 1, 2$ regardless of microstructures.

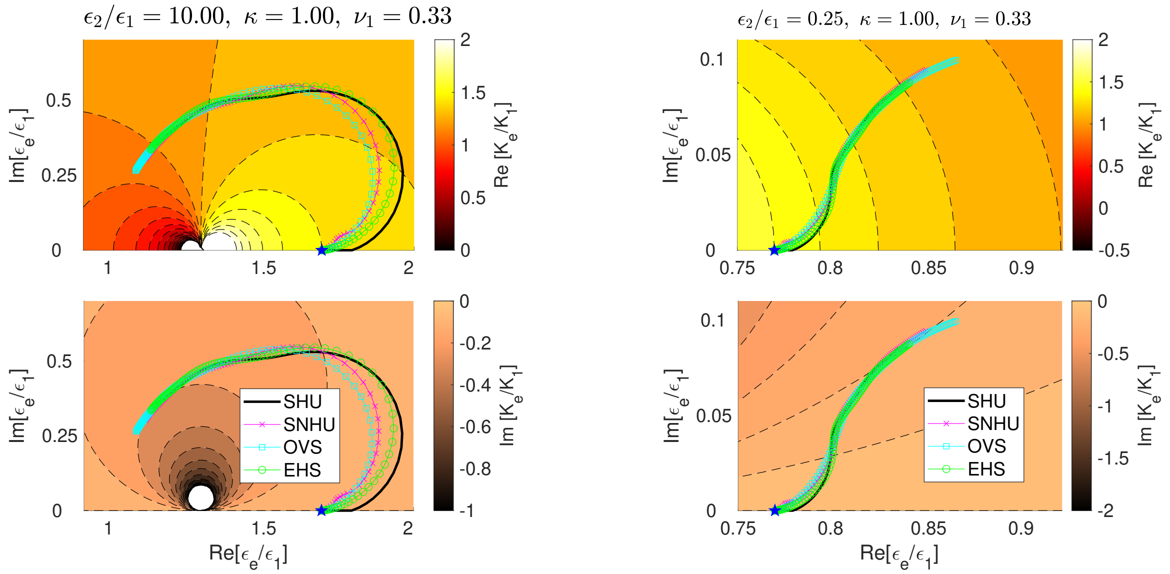


(a) (b)

FIG. S6. Cross-property relations between the effective dielectric constant $\epsilon_e$ and the effective bulk modulus $K_e$ in the case of a compressible matrix with $\nu_1 = 1/3$ containing an incompressible dispersed phase. The ratios of phase dielectric constants are (a) $\epsilon_2/\epsilon_1 = 10$ and (b) $\epsilon_2/\epsilon_1 = 0.25$. Contour plots, evaluated from Eq. (14) in the main text, represent the surface on which $\epsilon_e$ and the real (the upper panel) and the imaginary (the lower panel) parts of $K_e$ at a prescribed wavenumber $k_{L_1}$ should lie. We then overlap cross-property relations for four models of 3D disordered dispersions with $\phi_2 = 0.25$: stealthy hyperuniform (SHU), stealthy nonhyperuniform (SNHU), overlapping spheres (OVS), and equilibrium hard spheres (EHS). These curves start from the Hashin-Shtrikman bounds (blue stars) at $k_{L_1}a = 0$ to $k_{L_1}a = 5$.

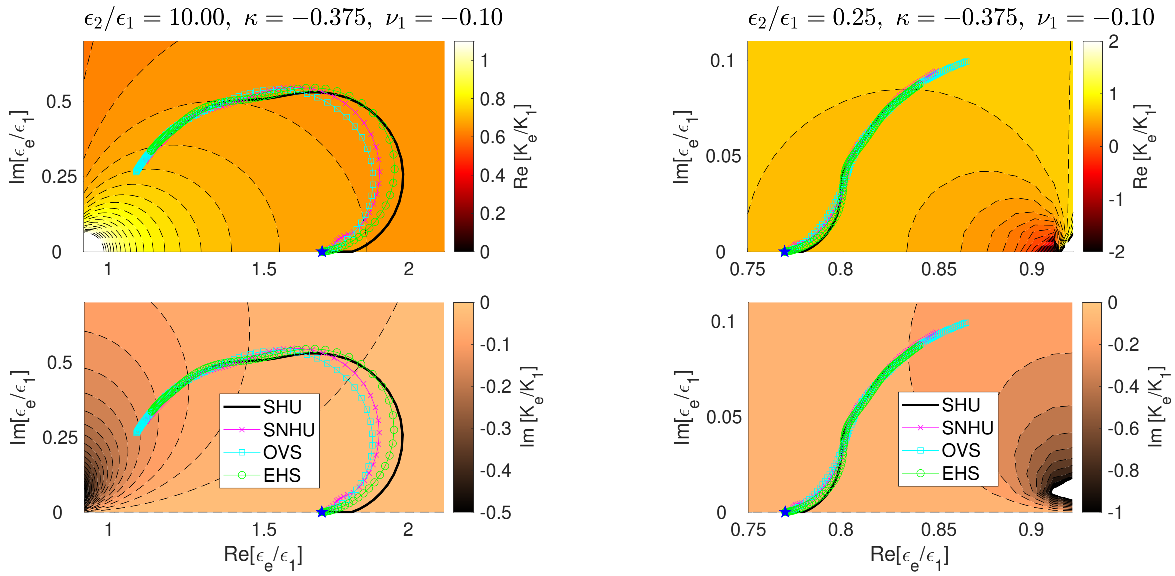


(a)

(b)

FIG. S7. Cross-property relations between the effective dielectric constant $\epsilon_e$ and the effective bulk modulus $K_e$ in the case of a compressible matrix with $\nu_1 = -0.1$ containing cavities. The ratios of phase dielectric constants are (a) $\epsilon_2/\epsilon_1 = 10$ and (b) $\epsilon_2/\epsilon_1 = 0.25$. The phase properties considered in (a) are identical to those in Fig. 4 in the main text. Contour plots, evaluated from Eq. (14) in the main text, represent the surface on which $\epsilon_e$ and the real (the upper panel) and the imaginary (the lower panel) parts of $K_e$ at a prescribed wavenumber $k_{L\,1}$ should lie. We then overlap cross-property relations for four models of 3D disordered dispersions with $\phi_2 = 0.25$: stealthy hyperuniform (SHU), stealthy nonhyperuniform (SNHU), overlapping spheres (OVS), and equilibrium hard spheres (EHS). These curves start from the Hashin-Shtrikman bounds (blue stars) at $k_{L\,1}\,a = 0$ to $k_{L\,1}\,a = 5$.

[1] S. Torquato, *Random Heterogeneous Materials: Microstructure and Macroscopic Properties*, Interdisciplinary Applied Mathematics (Springer Science & Business Media, 2002).
[2] P. Debye and A. M. Bueche, "Scattering by an inhomogeneous solid," J. Appl. Phys. **20**, 518–525 (1949).
[3] S. Torquato, "Effective electrical conductivity of two-phase disordered composite media," J. Appl. Phys. **58**, 3790–3797 (1985).
[4] O. U. Uche, F. H. Stillinger, and S. Torquato, "Constraints on collective density variables: Two dimensions," Phys. Rev. E **70**, 046122 (2004).
[5] R. D. Batten, F. H. Stillinger, and S. Torquato, "Classical disordered ground states: Super-ideal gases and stealth and equi-luminous materials," J. Appl. Phys. **104**, 033504 (2008).
[6] G. Zhang, F. H. Stillinger, and S. Torquato, "Ground states of stealthy hyperuniform potentials: I. Entropically favored configurations," Phys. Rev. E **92**, 022119 (2015).
[7] G. Zhang, F. H. Stillinger, and S. Torquato, "Can exotic disordered "stealthy" particle configurations tolerate arbitrarily large holes?" Soft Matter **13**, 6197–6207 (2017).
[8] M. C. Rechtsman and S. Torquato, "Effective dielectric tensor for electromagnetic wave propagation in random media," J. Appl. Phys. **103**, 084901 (2008).
[9] H. Moulinec and P. Suquet, "A numerical method for computing the overall response of nonlinear composites with complex microstructure," Comput. Methods Appl. Mech. Engrg. **157**, 69–94 (1998).
[10] D. J. Eyre and G. W. Milton, "A fast numerical scheme for computing the response of composites using grid refinement," Eur. Phys. J. Appl. Phys. **6**, 41–47 (1999).
[11] W. Shin and S. Fan, "Choice of the perfectly matched layer boundary condition for frequency-domain Maxwell's equations solvers," J. of Comp. Phys. **231**, 3406–3431 (2012).
[12] A. Sihvola, *Electromagnetic Mixing Formulas and Applications* (IET Digital Library, 1999).
[13] R. Ruppin, "Evaluation of extended Maxwell-Garnett theories," Opt. Commun. **182**, 273–279 (2000).
[14] A. Sprafke and J. Schilling, "9 - Non-resonant dielectric metamaterials," in *Dielectric Metamaterials*, Woodhead Publishing Series in Electronic and Optical Materials, edited by Igal Brener, Sheng Liu, Isabelle Staude, Jason Valentine, and Christopher Holloway

(Woodhead Publishing, 2020) pp. 249–288.

[15] C. O. Ao and J. A. Kong, "Analytical approximations in multiple scattering of electromagnetic waves by aligned dielectric spheroids," J. Opt. Soc. Am. A **19**, 1145–1156 (2002).

[16] O. Leseur, R. Pierrat, and R. Carminati, "High-density hyperuniform materials can be transparent," Optica **3**, 763–767 (2016).

[17] F. H. Kerr, "The scattering of a plane elastic wave by spherical elastic inclusions," Int. J. Eng. Sci. **30**, 169–186 (1992).
